# Supplementary material for: Inter-subject Deep Transfer Learning for Motor Imagery EEG Decoding
Source: arXiv:2103.05351 source file (2021-03-09)
Supplement: Supplementary file 1 [file appendix.tex]

%\appendix

% \begin{figure*}
% \centering
% \includegraphics[scale=0.53]{figure6.png}
% \caption{Eye artefact removal of blinks (left) and glances(right). There are two groups of figures, in which the left group shows the blink artefact removal and the right group shows the glance artefact removal. The upper-left pictures of both groups are the raw EEG. In the upper right and bottom left, EEG signals after filtered by the 4Hz high-pass filter and the EoG regression are shown. We can observe that it still remains some residuals of blink or glance artefacts respectively, when the high-pass filter or the EoG regression is applied alone. They were filtered out after using both methods, as shown in the bottom-right figures.}
% \label{figure6}
% \end{figure*}
